# Supplementary material for: Disentangled Planning and Control in Vision Based Robotics via Reward Machines
Source: arXiv:2012.14464 source file (2020-12-28)
Supplement: Supplementary file 1 [file supplemental.tex]

\section*{Considerations for CoRL2020 and the Pandemic}

% The CoRL 2020 organising committee and board acknowledge the challenges in producing high-quality experimental results during the social distance policies implemented in different parts of the world. Authors affected by these policies are encouraged to submit a one-page supplemental material explaining how their method will be experimentally validated with real data. 

% Papers with no real robot experimental results (and that could not rely on experimental datasets) should contain extensive experimentation in simulation. Those papers should explicitly detail why the authors believe their method will also work on real robots and explain the measures taken to support this claim (e.g., utilising more than one simulator). Reviewers will be requested to carefully consider empirical evidence in simulation on the basis of its generalisation properties to real scenarios.    

We have had no access to our real robot hardware for the last several months due to COVID-19, and were unable to run experiments outside of simulation.  We are confident that our method will generalize to real robot hardware.  We demonstrate how reward machines can significantly improve learning of vision-based RL policies on robot manipulation tasks.  The problem domain, model architecture, observation space, and action space utilized in this work are commonly used on real robots.  The type of feature detectors that are leveraged to create abstract states are inspired from features that are also already utilized on real robot systems. 

Our work is using a set of tasks, model architecture, observation space, action space whose different components overlap heavily with:
\begin{itemize}
    \item Zakka, Kevin, et al. "Form2fit: Learning shape priors for generalizable assembly from disassembly." arXiv preprint arXiv:1910.13675 (2019).
    \item Zeng, Andy, et al. "Learning synergies between pushing and grasping with self-supervised deep reinforcement learning." 2018 IEEE/RSJ International Conference on Intelligent Robots and Systems (IROS). IEEE, 2018.
    \item Zeng, Andy, et al. "Tossingbot: Learning to throw arbitrary objects with residual physics." IEEE Transactions on Robotics (2020).
\end{itemize}

These works all have extensive real robot experimental sections. Our 3 block kitting task is representative of many real world tasks such as the kitting tasks in Form2Fit.  Our overhead observation space, and our parameterization of pick and place actions via Q-value heatmaps is also closely related to the above works.  

Our work also utilizes feature detectors to determine what the current abstract state is.  These feature detectors relate to whether or not an object is present in the gripper, on the table, or in the correct kit location.  We argue that obtaining these signals on real robot hardware is reasonable, and already commonly done.  Many are simple features, like whether or not something is contained in the gripper. Other features relate to classification and pose estimation of table top objects. There is a large, mature body of literature in this area. Some recent examples include:
\begin{itemize}
    \item Tremblay, Jonathan, et al. "Deep object pose estimation for semantic robotic grasping of household objects." arXiv preprint arXiv:1809.10790 (2018).
    \item Zeng, Zhen, et al. "Semantic mapping with simultaneous object detection and localization." 2018 IEEE/RSJ International Conference on Intelligent Robots and Systems (IROS). IEEE, 2018.
    \item Akkaya, Ilge, et al. "Solving rubik's cube with a robot hand." arXiv preprint arXiv:1910.07113 (2019).
    \item Zeng, Andy, et al. "Robotic pick-and-place of novel objects in clutter with multi-affordance grasping and cross-domain image matching." 2018 IEEE international conference on robotics and automation (ICRA). IEEE, 2018.
\end{itemize}

The above works are able to do pose estimation, and object classification on real robot hardware.  Our work, when operating on real hardware leverages the same ideas. These works demonstrate that feature detectors are already required to enable complex robot behaviors. Our work is not required additional features compared to the in hand classifiers and state estimators used above.  Our work is providing a more sophisticated way to leverage these signals and make learning of vision based RL policies more effective.
